# Supplementary material for: Cooperation Through Indirect Reciprocity in Child-Robot Interactions
Source: arXiv:2512.20621 source file (2025-11-07)
Supplement: Supplementary file 1 [file Supplementary_Material.pdf]

# Supplementary Material: Cooperation Through Indirect Reciprocity in Child-Robot Interactions

Isabel Neto*[1], Alexandre S. Pires*[2], Filipa Correia[3] and Fernando P. Santos[2]

[1]Lasige, Faculdade de Ciências, Universidade de Lisboa, Lisbon, Portugal
[2]Institute of Informatics, University of Amsterdam, Amsterdam, The Netherlands
[3]Interactive Technologies Institute, Instituto Superior Técnico, Universidade de Lisboa, Lisbon, Portugal

November 7, 2025

## 1 Hyperparameter selection

In all our experiments, we reported our results using the parameters that maximise cooperation under a mutual cooperation benefit of $b = 2.0$, as used in the user study, and $p = 0.81$ and $q = 0.36$, following the experimentally observed values. In Figure 1, we present the cooperation index of $\epsilon$-greedy and UCB1 under different hyperparameters. We exclude Thompson Sampling as it is not parameterised.

To better understand the impacts of different parametrisations, in Figures 2 and 3, similar to the main text, we present the levels of cooperation of each algorithm under different hyperparameters. In particular, we focus on a higher $\epsilon$, $\epsilon = 1/32$ for $\epsilon$-greedy, promoting higher exploration, and a lower incentive to explore, $c = 1$, in UCB1. Under a higher $\epsilon$, $\epsilon$-greedy achieves lower overall cooperation, and gains a higher sensitivity to $q$, as predicted by the theoretical threshold $\left((1 - \frac{\epsilon}{2})p + \frac{\epsilon}{2}q\right)(b + 3) > 3$. UCB1 requires a lower $b$ to achieve cooperation, yet reaches lower levels of cooperation at a high $b$. Furthermore, at a lower $c$, UCB1 will value underexplored actions less, and thus is less prone to defect if cooperation is beneficial, reducing the risk of incorrectly valuing defection when it cooperated in a prior round. As such, despite achieving lower overall cooperation, UCB1 loses its sensitivity to a low $q$, allowing it to sustain cooperation facing *Trust Cooperators* (*TC*, $p = 1$, $q = 0$).

*Equal contribution

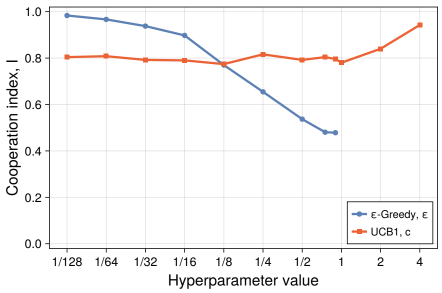


Figure 1: Cooperation index, $I$, across hyperparameters for $\epsilon$-greedy ($\epsilon$) and UCB1 ($c$). We observe that $\epsilon = 1/128$ and $c = 4$ maximise cooperation under the experimentally observed $p$ and $q$, and as such were selected for all experiments. Parameters used: $p = 0.81$, $q = 0.36$.

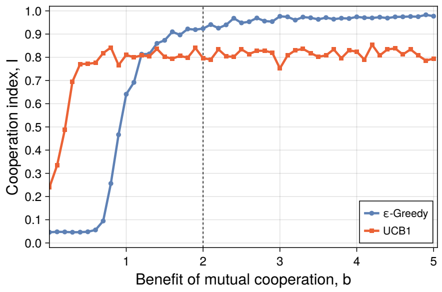


Figure 2: Cooperation index, $I$, for various levels of cooperation benefit, $b$, at higher exploration rates for $\epsilon$-greedy and lower value of exploration for UCB1. The dashed line, at $b = 2$, indicates the benefit of mutual cooperation used in the experimental setting (how many additional Lego pieces are given). Compared to the lower $c$ used in the main text, UCB1 stabilises at lower mutual cooperation benefit values, yet achieves lower levels of cooperation at high $b$. $\epsilon$-greedy with a higher $\epsilon$, on the other hand, requires a higher $b$ to converge and has reduced maximum cooperation. Parameters used: $p = 0.81$, $q = 0.36$, $\epsilon = 1/32$, $c = 1$.

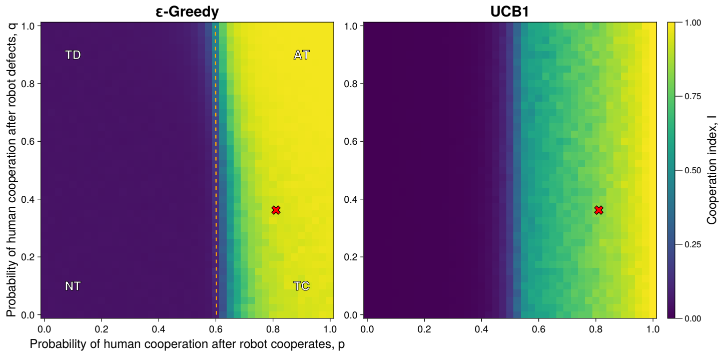


Figure 3: Cooperation index, $I$, varying $p$ and $q$, at higher exploration rates for $\epsilon$-greedy and lower value of exploration for UCB1. The red cross indicates the experimental value found for $p$ and $q$ ($p = \hat{p} = 0.81$, $q = \hat{q} = 0.36$). Labels indicate the pure strategy used by humans at that point: *Always Trust, AT* ($p = 1, q = 1$), which always cooperates; *Never Trust, NT* $(0, 0)$, which always defects; *Trust Cooperators, TC* $(1, 0)$, which only cooperates if the algorithm previously cooperated; and *Trust Defectors, TD* $(0, 1)$, which only cooperates after observing a defection. The vertical line in $\epsilon$-greedy indicates its theoretical threshold for cooperation to dominate defection (see Methods of the main text). Compared to the lower $\epsilon$ used in the main text, a higher $\epsilon$ leads to a higher uncertainty from the algorithm, degrading cooperation across the theoretical threshold and increasing the dependency on $q$. In UCB1, a lower $c$ discourages exploration, increasing consistency. As such, UCB1 loses sensitivity to $q$ and instead presents a threshold similar to $\epsilon$-greedy. Parameters used: $b = 2$, $\epsilon = 1/32$, $c = 1$.

# 2 Long-term human cooperation

Similar to how the cooperation index of the algorithm is measured by the fraction of times the algorithm opts to cooperate, we also measure the fraction of times the algorithm receives cooperation, $I^R$. In Figure 4, we study human cooperation with the algorithm as we vary $b$, the benefit of mutual cooperation. As mentioned in the main text, by definition, $I^R$ is bounded by $min(p, q) \leq I^R \leq max(p, q)$, leading to a maximum value of $p$ ($q$) when always cooperating (defecting). Importantly, we observe that differences in the cooperation levels of the algorithm are reflected, yet attenuated, in the cooperation received by the algorithm.

Similarly, in Figure 5, we study human cooperation under different regimes of $p$ and $q$. This allows us to understand the impact of the algorithm in different cultural regimes. We observe that cooperation is much more prevalent across the entire strategy space than in the case of the algorithm, due to the previously explained bounds in human cooperation. In general, we also observe that the

regions that maximise cooperation in the algorithm also maximise it in the predicted human behaviour. However, there are also high levels of cooperation in other regions, particularly *Trust Defectors* ($TD$, $p = 0$, $q = 1$), as a result of low cooperation from the algorithm, where under this theoretical region, algorithms that defect are optimal.

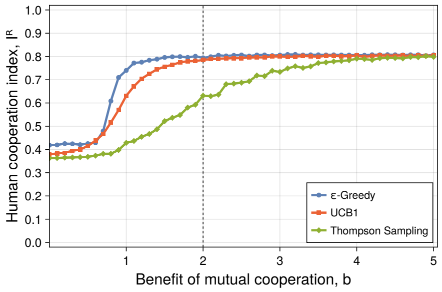


Figure 4: Human cooperation index, $I^R$, at various levels of cooperation benefit, $b$, for the three algorithms we utilise to simulate the robot learning to play with children. The dashed line, at $b = 2$, indicates the benefit of mutual cooperation used in the experimental setting (how many additional Lego pieces are given). We observe that, as a result of the cooperation rate of the algorithm, cooperation is upper-bounded at $p$ and lower-bounded at $q$, diminishing the effect of the algorithm on human cooperation. Parameters used: $p = 0.81$, $q = 0.36$, $\epsilon = 1/128$, $c = 4$.

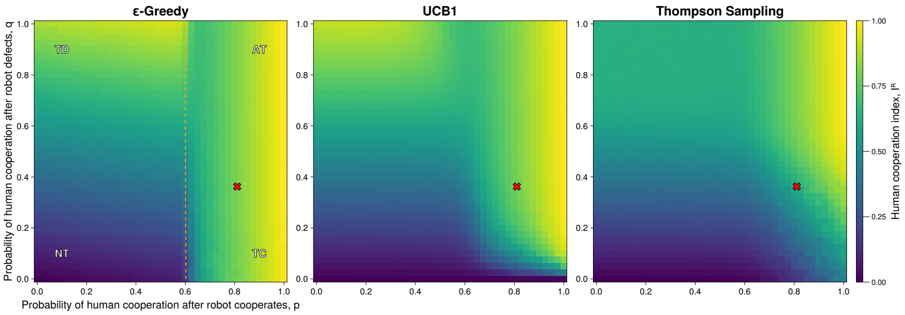


Figure 5: Human cooperation index, $I^R$, varying $p$ and $q$, for the three learning algorithms used. The red cross indicates the experimental value found ($p = \hat{p} = 0.81$, $q = \hat{q} = 0.36$). Labels indicate the pure strategy used by humans at that point: *Always Trust, AT* ($p = 1, q = 1$), which always cooperates; *Never Trust, NT* $(0, 0)$, which always defects; *Trust Cooperators, TC* $(1, 0)$, which only cooperates if the algorithm previously cooperated; and *Trust Defectors, TD* $(0, 1)$, which only cooperates after observing a defection. The vertical line in $\epsilon$-greedy indicates its theoretical threshold for the algorithm to adopt cooperation instead of defection (see Methods in main text). We observe how cooperation can persist in areas where the algorithm does not cooperate, such as *TD*. Yet, around *AT* and *TC* cooperation is promoted by cooperative algorithms. Parameters used: $b = 2$, $\epsilon = 1/128$, $c = 4$.

# 3 Time convergence of each algorithm

An important factor to consider when utilising a learning agent is the time it takes for the agent to learn. While an algorithm might perform optimally in certain environments, during the time needed to adapt to other environments, the interactions of the algorithm will still impact its users. As such, algorithms should also be selected considering their time to learn. Furthermore, not all algorithms learn at the same pace and with similar dynamics in the resulting cooperation.

In Figure 6 we fix $b$, $p$ and $q$ and study cooperation throughout rounds, averaged over 5000 simulations. We observe important details regarding the learning rate of each algorithm: $\epsilon$-greedy converges in the first few rounds, while Thompson Sampling takes around 250 rounds to converge. On the other hand, cooperation under UCB1 is still increasing after 2500 rounds. Notably, after a long learning period, UCB1 is able to surpass $\epsilon$-greedy in cooperation. Yet, during the first few rounds, it is considerably worse. These different learning rates should be considered when selecting which algorithm to use.

To study the behaviour across the full range of human strategies, in Figure 7, we present the cooperation index of each algorithm across different numbers of rounds (200, 2000, and 10000). Importantly, we do not observe the same patterns of learning across all algorithms. In particular, $\epsilon$-greedy starts highly

cooperative across the entire region of strategies, later evolving to the theoretical $p$ threshold of cooperation by reducing cooperation outside of this range. Conversely, UCB and Thompson Sampling instead start with reduced regions of cooperation, that get more prominent as the algorithm learns. While all algorithms present areas where cooperation decreases throughout learning, $\epsilon$-greedy shows a greater area where this happens. This is significant when considering the first interactions that individuals might have with the algorithm, which can shape their perception and response.

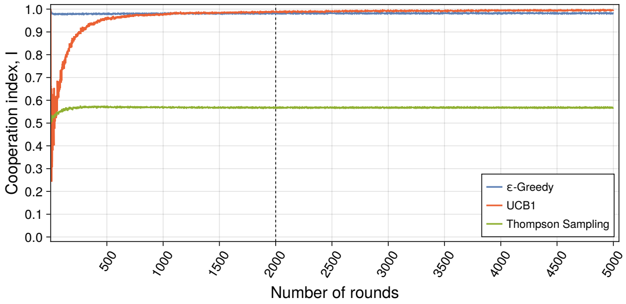


Figure 6: Cooperation index, $I$, across rounds, as each algorithm learns. The black vertical line, at 2000 rounds, indicates the value used in the main paper. We observe that learning differs between algorithms, with UCB1 taking the longest to converge. Outside of the first rounds of UCB1, learning is stable and cooperation generally increases or is sustained through time. Parameters used: $p = 0.81$, $q = 0.36$, $b = 2$, $\epsilon = 1/128$, $c = 4$.

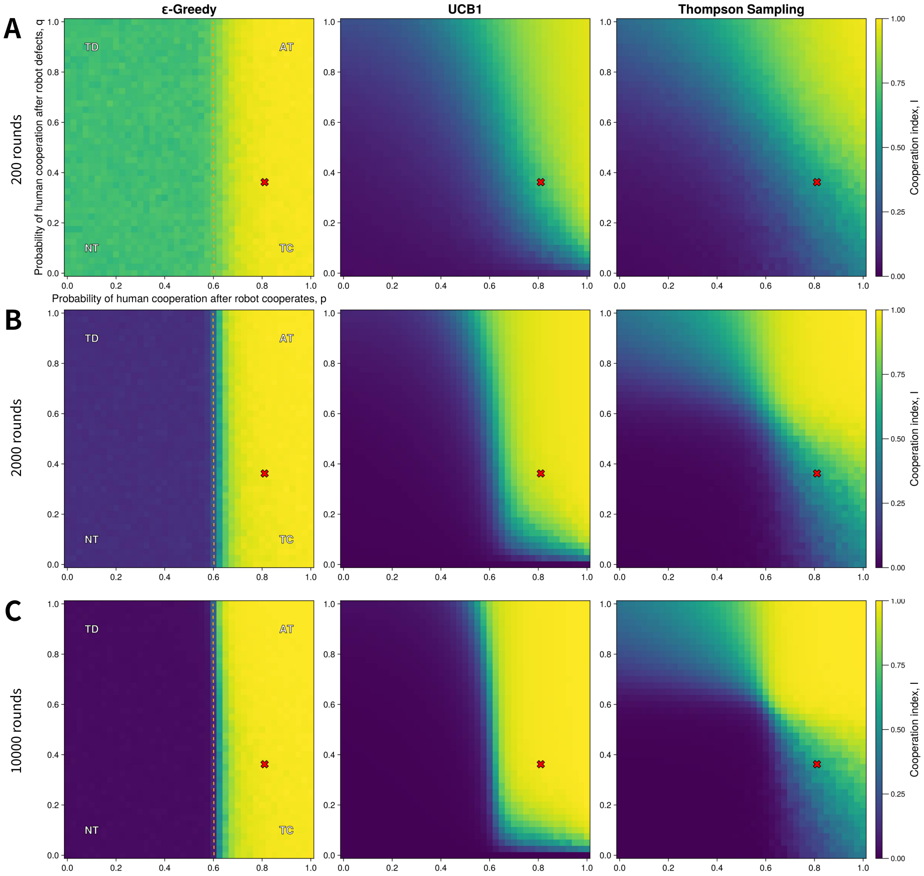


Figure 7: Cooperation index, $I$, varying $p$ and $q$, for the three learning algorithms used, at different numbers of rounds (**A** 200 rounds, **B** 2000 rounds and **C** 10000 rounds). The red cross indicates the experimental value found ($p = \hat{p} = 0.81$, $q = \hat{q} = 0.36$). Labels indicate the pure strategy used by humans at that point: *Always Trust, AT* ($p = 1, q = 1$), which always cooperates; *Never Trust, NT* $(0, 0)$, which always defects; *Trust Cooperators, TC* $(1, 0)$, which only cooperates if the algorithm previously cooperated; and *Trust Defectors, TD* $(0, 1)$, which only cooperates after observing a defection. The vertical line in $\epsilon$-greedy indicates its theoretical threshold for cooperation to dominate defection (see Methods in main text). We observe that in $\epsilon$-greedy, cooperation under low $p$ is reduced throughout training, as the algorithm learns to maximise payoff. Under UCB1 and Thompson Sampling, a region with high cooperation is formed throughout learning, and uncooperative regions face only small decreases as the algorithm stabilises. Parameters used: $b = 2$, $\epsilon = 1/128$, $c = 4$.
